# Supplementary material for: Machine-Learning-Accelerated Surface Exploration of Reconstructed BiVO$_{4}$(010) and Characterization of Their Aqueous Interfaces
Source: arXiv:2412.08126 source file (2024-12-11)
Supplement: Supplementary file 1 [file SI.pdf]

# Machine-Learning-Accelerated Surface Exploration of Reconstructed $BiVO_4(010)$ and Characterization of Their Aqueous Interfaces

Yonghyuk Lee[†] and Taehun Lee[*,‡,¶]

†*Department of Chemistry and Biochemistry, University of California Los Angeles, Los Angeles, California, 90095, United States*

‡*Division of Advanced Materials Engineering, Jeonbuk National University, Jeonju 54896, Republic of Korea*

¶*Hydrogen and Fuel Cell Research Center, Jeonbuk National University, Jeonbuk, 54896, Republic of Korea*

E-mail: taehun.lee@jbnu.ac.kr

# Methods

## Gaussian Approximation Potential

Gaussian Approximation Potentials (GAPs) represent a prominent category of machine learning interatomic potentials (MLIPs), leveraging a sparse variant of Gaussian process regression.[1–3] In this study, we train a $BiVO_4$ GAP model following the training protocol detailed in previous research,[4] which outlines the formalism and iterative training processes for surface unit cells. To avoid redundancy, we provide a succinct overview and direct the reader to the original source for an in-depth explanation.

GAPs function as efficient surrogates for the potential energy surface (PES) of a system, enabling the calculation of the total energy, $E_{\mathrm{GAP}}$, based on the atomic coordinates $\mathbf{X_n}$. The energy expression is given by:

$$\begin{aligned} E_{\mathrm{GAP}}(\mathbf{X_n}) = & \underbrace{\sum_{i,j} \delta_{\mathrm{2B}}^2 \sum_{m=1}^{M_{\mathrm{2B}}} c_{m,\mathrm{2B}} k_{\mathrm{2B}}(r_{ij}, r_m)}_{E_{\mathrm{2B}}} \\ & + \underbrace{\sum_{i} \delta_{\mathrm{MB}}^2 \sum_{m=1}^{M_{\mathrm{MB}}} c_{m,\mathrm{MB}} k_{\mathrm{MB}}(\boldsymbol{\chi}_i, \boldsymbol{\chi}_m)}_{E_{\mathrm{MB}}} \quad . \end{aligned} \tag{S1}$$

This formulation comprises two main components: the two-body (2B) energy, $E_{\mathrm{2B}}$, and the many-body (MB) energy, $E_{\mathrm{MB}}$. The 2B energy arises from pairwise interactions between atoms $(i, j)$, while the MB energy accounts for more complex interactions involving multiple atoms within the local atomic environments of the system, with atom $i$ at the center. The calculations incorporate a set of $M_{\mathrm{2B/MB}}$ representative data points, characterized by regression coefficients $c_{m,\mathrm{2B/MB}}$ and kernel functions $k_{\mathrm{2B/MB}}$. These kernel functions quantify the similarity between local geometric descriptors derived from $\mathbf{X_n}$.

The 2B contribution primarily utilizes interatomic distances $r_{ij}$, processed through a squared exponential (Gaussian) kernel, up to a defined cutoff radius $r_{\mathrm{cut}}$. In contrast, the MB

contribution employs descriptors based on the Smooth Overlap of Atomic Positions (SOAP),[5] which provide invariant vectorial representations of the local atomic environment $\boldsymbol{\chi}_i$. These descriptors are integrated into a dot product kernel. Key technical hyperparameters used herein, such as the relative weights $\delta_{\mathrm{2B/MB}}$, SOAP and kernel parameters, and the radial cutoff $r_{\mathrm{cut}}$ (refer to Figure S1), are specified in Table S1.

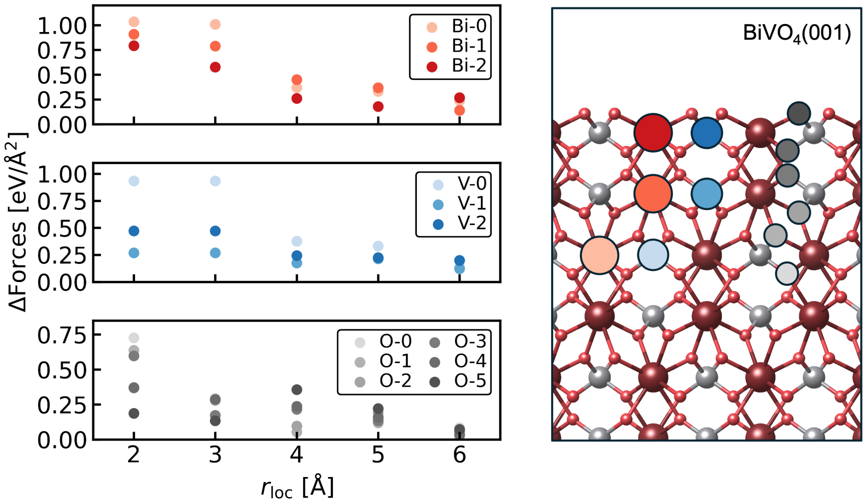


Figure S1: Force locality test for the $BiVO_4$(010) stoichiometric surface. The induced force on a given central atom upon displacement of atoms outside a radius $r_{\mathrm{loc}}$ is shown. Three, three, and six different central atoms for Bi, V, and O, respectively, are considered from the outermost to the inner atomic layers in the slab, as illustrated in the right panel.

Table S1: Hyperparameters used for the GAP model in this work.

| Description | Symbol | 2B | SOAP |
|---|---|---|---|
| Cutoff (Å) | $r_{\mathrm{cut}}$ | 5.0 | |
| Kernel width (Å) | $\sigma$ | 1.0 | 0.5 |
| Scaling factor (eV) | $\delta$ | 0.372 | 0.108 |
| SOAP basis | $n_{\mathrm{max}}/l_{\mathrm{max}}$ | - | 8/4 |
| Number of sparse points | $M$ | 25 | 2000 |
| Kernel exponent | $\zeta$ | - | 4 |
| Regularization factors | $\sigma_{\varepsilon}$ (eV)/$\sigma_{\mathrm{f}}$ (eV/Å) | 0.001/0.01 | |

To refine the GAP further, an iterative workflow involving density functional theory (DFT) data is employed.[4] This process starts with a minimal initial set of training structures, manually curated by the researcher. In detail, the initial training set was constructed using DFT-calculated data, including $O_2$ dimers with varying O-O bond lengths, and $BiVO_4$ bulk structures. These bulk structures included both fully optimized unit cells and $(2 \times 2 \times 1)$ supercells with constrained lattice constants, where internal coordinates were either optimized or deliberately displaced. Additionally, the training set incorporated 13 inequivalent $(1 \times 1)$ surface configurations derived from straightforward bulk truncations. For each truncation, both the raw bulk-truncated geometries and their DFT-refined counterparts were included in the dataset. The preliminary GAP is then used to conduct various global geometry optimization runs, exploring a wide array of surface stoichiometries within the specified surface unit cell. The resulting configurations are evaluated against existing training structures using a kernel distance metric, defined as:

$$\kappa(A, B) = \sqrt{2 - 2\min_{\substack{a \in A \\ b \in B}}(k_{\mathrm{MB}}(\boldsymbol{\chi}_a, \boldsymbol{\chi}_b))} \quad , \tag{S2}$$

where $\kappa(A, B)$ assesses the presence of novel atomic environments by identifying the minimal similarity $k_{\mathrm{MB}}(\boldsymbol{\chi}_a, \boldsymbol{\chi}_b)$ between any atoms $a \in A$ and $b \in B$. A critical threshold value, $\kappa_{\mathrm{crit}} = 0.075$, is employed to determine whether a newly encountered configuration is distinct enough to warrant its inclusion in the training set, followed by local DFT optimization.

The iterative refinement cycle continues with the retraining of the GAP whenever new structures are added to the training set. This process repeats until either no further novel structures are identified or the out-of-sample error for the most recently added structures drops below a specified threshold. In this study, we employ a force accuracy threshold of 250 meV/Å, which corresponds to the average locality error for a 5 Å cutoff radius.

Upon completion of the training iterations, the final set of training structures comprises the output of a multi-generation surface structure exploration. If the training concludes

because the GAP has sufficiently captured all relevant local geometric motifs, all lowest-energy structures identified in both preceding and subsequent global geometry optimization runs are further refined using DFT geometry optimizations. The lowest-energy structures discussed in this paper correspond to these DFT-optimized geometries and their associated energetics.

We summarize the active learning (AL) protocol and the quality of the resulting GAP and training set in Figure S2.

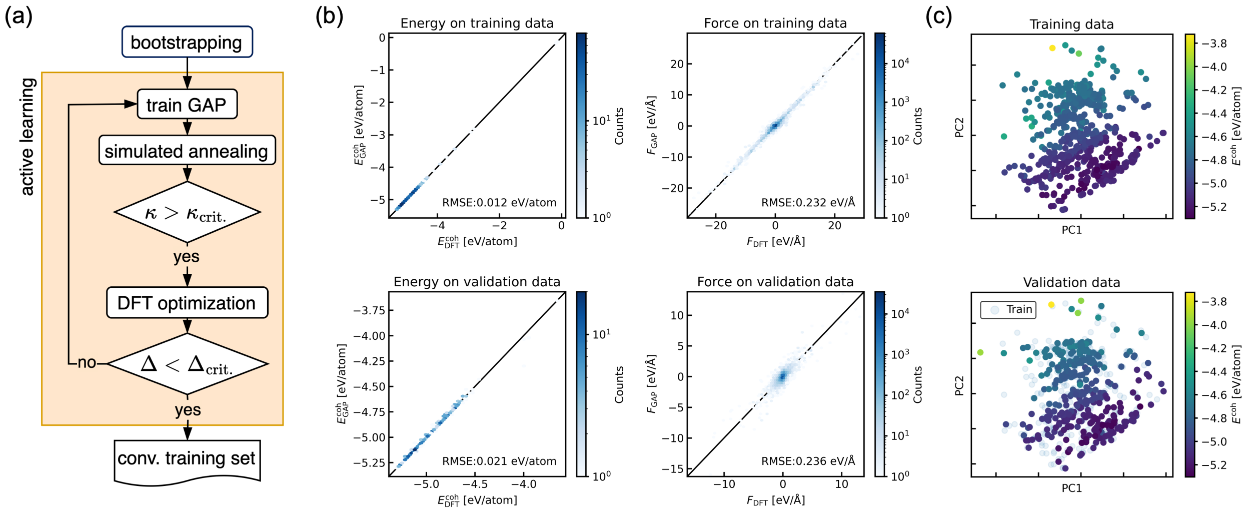


Figure S2: (a) A summarized flowchart of the active learning (AL) protocol used to obtain a converged training set for the Gaussian Approximation Potential (GAP) machine-learning interatomic potential. This flowchart outlines the iterative steps involved in the selection and refinement of training data, from the bootstrapping DFT calculations to the integration of newly identified structures. (b) Energy and force correlation plots comparing the results from DFT calculations and the GAP model. The root mean square error (RMSE) values are provided in each figure to quantify the accuracy of the GAP relative to the DFT data. (c) A principal component analysis (PCA) of the structures in the final training and validation datasets. The PCA visualizes the distribution of structural configurations and highlights the diversity captured in the datasets. In the bottom panel, which represents the validation data, the training data points are also shown as pale blue circles, emphasizing the similarity and coverage between the training and validation datasets.

## Simulated Annealing

The global geometry optimization using GAP is conducted through a molecular dynamics (MD) based simulated annealing (SA) protocol. The MD simulations are performed with the LAMMPS code,[6] utilizing the velocity Verlet algorithm[7] with time steps of 1 fs. A canonical $NVT$ ensemble is employed, with temperature control achieved via a Berendsen thermostat[8] for efficient thermal regulation. In the SA protocol, the system is heated from 200 to 800 K and then quenched back to 200 K at a constant heating and cooling rate of 1.2 K/ps. After each SA cycle, the resulting finite-temperature structure undergoes full geometry optimization using conjugate gradient minimization, adhering to the same convergence threshold applied in subsequent DFT calculations.

To mitigate the desorption of stable molecular motifs from the surface during the high-temperature phase of the SA, a harmonic repulsive potential is applied. This potential begins at the topmost layer of the surface slab and increases linearly, reaching a maximum value of 10 eV at a height of 10 Å above the surface. During the cool-down phase of the SA, the potential is gradually reduced and completely removed by the time the cool-down is complete and the geometry optimization begins. This approach ensures that the confinement potential does not influence the final structures or their energetics, while still permitting lateral mass transfer of surface species during the high-temperature phase of the SA.

## Density-functional theory calculations

All DFT calculations are performed using a plane-wave basis set and optimized norm-conserving Vanderbilt pseudopotentials (ONCVPSP),[9] as implemented in the Quantum ESPRESSO software package.[10] To efficiently generate data for training the GAP within the active learning workflow, all structures in the training set are calculated using the semi-local Perdew-Burke-Ernzerhof (PBE) functional[11] to describe electronic exchange and correlation. The kinetic energy cutoff for the wave function expansion is set to 90 Ry, while a charge density cutoff of 360 Ry is used. Brillouin-zone integrations are performed using a k-point grid with reciprocal distances of 0.05 $Å^{-1}$, corresponding to a $(6 \times 6 \times 4)$ k-point grid for the tetragonal ($I4_1/a$) bulk $BiVO_4$.

For benchmarking and comparison, we employ the DFT+$U_{\text{eff}}$[12] optimized lattice parameters for bulk $BiVO_4$ from Ref. 13, allowing us to effectively align our results with closely related studies by the same authors.[14–16] Geometry optimizations in slab calculations are carried out using Broyden-Fletcher-Goldfarb-Shanno (BFGS) minimization,[17–19] with convergence criteria set to residual changes in total energy below $1.4 \times 10^{-2}$ meV and force components below 0.3 meV/Å. Periodic boundary conditions are employed in slab calculations with a minimum vacuum separation of 20 Å. Symmetric slab models comprising at least ten trilayers of $BiVO_4$ units are used within the $(1 \times 1)$ surface unit cell of (010) facets.

The global minimum structures obtained using the PBE functional for all stoichiometric surfaces are further optimized using dielectric-dependent PBE0 hybrid functional calculations implemented in CP2K code[20] to understand more accurate and reliable properties for electrochemical conditions. The PBE0 calculations were accelerated using the Truncated Coulomb and Long Range Correction (PBE0-TC-LRC) method[21] along with the auxiliary density matrix method.[22] Here, we use the fraction of Fock exchange ($\alpha$) set to $\alpha = 1/\epsilon_\infty = 0.22$, which is appropriate to reproduce the experimental band gap (about 2.6 eV).[23,24] We employed Goedecker-Teter-Hutter (GTH) pseudopotentials[25] to describe core-valence interactions, using molecularly optimized (MOLOPT) double-$\zeta$ polarized basis

sets for Bi, O, and V, and triple-$\zeta$ basis sets for H atoms.[26] A cutoff of 600 Ry was used to expand the electron density in plane waves.

To ensure that no potential global minimum structures are overlooked due to energy inversions between energetically comparable structures from PBE and PBE0, we additionally calculate the five most stable PBE local minima structures for surface stoichiometries identified as stable in the Pourbaix diagram. Specifically, we employ $p(2 \times 2)$ surface supercell of these structures to further allow reconstructions to possibly take place due to the higher degree of freedom.

For the PBE0 global minimum structures that are Pourbaix-diagram stable ($\mathbf{t}$-$BiVO_4$, $\mathbf{t}$-$BiO_2$, $\mathbf{t}$-$BiO_3$, $\mathbf{t}$-$VO_2$, $\mathbf{t}$-$VO_4$), we build interfaces with a 56-water model, using the initial water configuration from the previous theoretical study on the $BiVO_4$(010)-water interface.[27] Consequently, each simulation box had a water layer at least 15 Å thick, matching the experimental water density (see Figure S4). We then run *ab initio* MD (*ai*MD) with the same computational setup (CP2K with PBE0) for at least 7 ps with a time step of 0.5 fs in the canonical ($NVT$) ensemble. These simulations employed the D3 method[28] to account for van der Waals interactions, with the temperature set at 350 K to ensure proper diffusive motion of the liquid water. Geometric properties of the aqueous interface along the *ai*MD trajectories were analyzed using the neighbor module in the Atomic Simulation Environment (ASE).[29]

## Electrochemical stability

To explore the relative stability of $BiVO_4$ surfaces under electrochemical conditions, we calculated the Pourbaix diagram following the methods described in earlier studies.[30,31] We utilized ab initio thermodynamics to assess the relative stability of surface structures with varying chemical compositions.[32,33] The potential- and pH-dependent surface free energy $\gamma_{\rm surf}^{(010),\nu_i}$ of a (010)-oriented structure with a chemical composition $\nu_i$ is determined by

$$\gamma_{\rm surf}^{(010),\nu_i}(U,{\rm pH}) = \frac{1}{2A^{(010)}}\left[G_{\rm surf}^{(010),\nu_i} - \sum_i \nu_i\mu_i\right] \quad , \tag{S3}$$

where $G_{\rm surf}^{(010),\nu_i}$ represents the Gibbs free energy of the surface system, modeled using a symmetric slab within a supercell with surface unit cell area $A^{(010)}$. The chemical composition is characterized by $\nu_i$, denoting the number of atoms of various species $i$ (=Bi, V, O), while $\mu_i$ stands for the chemical potential of each species present. Assuming equilibrium between the surface and the underlying bulk $BiVO_4$ constrains the chemical potentials of Bi, V, and O to the Gibbs free energy (per formula unit) of bulk $BiVO_4$ (i.e., $G_{\rm BiVO_4,bulk} = \mu_{\rm Bi} + \mu_{\rm V} + 4\mu_{\rm O}$). The chemical potential of oxygen, $\mu_{\rm O}$, is determined by the aqueous environment, $\mu_{\rm O} = \mu_{\rm H_2O} - 2\mu_{\rm H}$. In Equation S3, the solid-state Gibbs free energies, $G_{\rm surf}^{(010),\nu_i}$ and $G_{\rm BiVO_4,bulk}$, are approximated by their corresponding DFT total energies.[34]

The chemical potential of $H_2O$ is calculated as

$$\mu_{\rm H_2O} = E_{\rm H_2O,molc} + F_{\rm H_2O}^{\rm vib} + \Delta\mu_{\rm liquid-gas} \quad , \tag{S4}$$

where $E_{\rm H_2O,molc}$ is the total energy of an isolated $H_2O$ molecule, and $\Delta\mu_{\rm liquid-gas} = -0.09$ eV[35] represents the Gibbs free energy difference between water in its liquid state and gas phase under standard conditions. $F^{\rm vib}$ is the vibrational free energy contribution, which is calculated as

$$F^{\rm vib} = E_{\rm ZPE} + \int C_p {\rm d}T - T\Delta S \quad , \tag{S5}$$

where $E_{\rm ZPE}$ is the zero-point energy,[36,37] $C_p$ is the heat capacity at constant pressure, and $\Delta S$ is the vibrational entropy of the system.[38]

Using the concept of a computational hydrogen electrode (CHE),[39] $\mu_{\rm H}$ is connected to the applied potential $U$ with reference to the RHE as follows:

$$\mu_{\rm H} = \frac{1}{2}\left(E_{\rm H_2,molc} + F^{\rm vib}_{\rm H_2}\right) + eU_{\rm RHE} \quad , \tag{S6}$$

which can also be related to the working conditions of $U$ and pH with reference to the standard hydrogen electrode (SHE):

$$\mu_{\rm H} = \frac{1}{2}\left(E_{\rm H_2,molc} + F^{\rm vib}_{\rm H_2}\right) + eU_{\rm SHE} - k_{\rm B}T\log_{10}({\rm pH}) \quad . \tag{S7}$$

Thus, $\mu_{\rm O}$ is defined as

$$\begin{aligned}\mu_{\rm O} &= \mu_{\rm H_2O} - 2\mu_{\rm H} \\ &= E_{\rm H_2O,molc} + F^{\rm vib}_{\rm H_2O} + \Delta\mu_{\rm liquid-gas} - \left(E_{\rm H_2,molc} + F^{\rm vib}_{\rm H_2} + 2eU_{\rm RHE}\right)\end{aligned} \tag{S8}$$

We assume a room temperature of $T = 298.15$ K, which corresponds to the operating temperature of the photocatalytic device.

In this framework, $\mu_{\rm Bi}$ and $\mu_{\rm V}$ are interdependent, given that $\mu_{\rm Bi}+\mu_{\rm V} = G_{\rm BiVO_4,bulk}-4\mu_{\rm O}$. We consider two distinct electrolyte conditions based on the ionic concentrations of either $C_{\rm Bi^{3+}}$ or $C_{\rm V^{2+}}$, each assumed to be $10^{-6}$ M. The CHE concept is also extended to ions, where the typical redox couple, represented as $\rm M_s \leftrightarrow M^{n+} + ne^-$, yields an electrochemical potential of

$$\mu_{\rm M^{n+},aq} + n\mu_{e^-} = G_{\rm Bi,s} - ne\left(U_{\rm SHE} - U^0\right) - k_{\rm B}T\log_{10}[C_{\rm M^{n+}}] \quad , \tag{S9}$$

where $U^0$ is the standard reduction potential of the metal relative to $U_{\rm SHE}$. The reduction

potentials for Bi and V[40–42] used here are

$$\begin{aligned} &Bi^{3+} + 3e^- \leftrightarrow Bi(s) \quad \Delta G = 0.308 \text{ V} \\ &V^{2+} + 2e^- \leftrightarrow V(s) \quad \Delta G = -1.175 \text{ V} \quad . \end{aligned} \tag{S10}$$

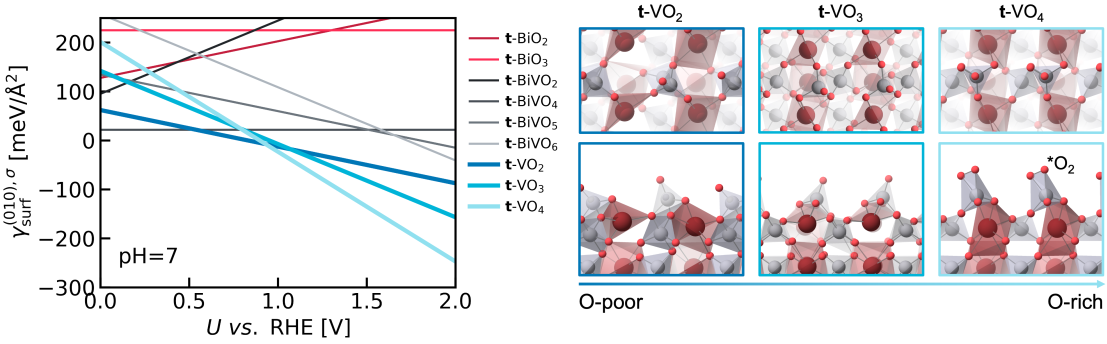


Figure S3: (left) Calculated surface phase diagram at pH= 7 under the V-rich ionic condition ($V^{2+}$(aq) concentration: $10^{-6}$ M). (right) Atomic structures of V-rich surfaces. Bi, V, and O atoms are represented by purple, gray, and red spheres, respectively. $BiO_n$ and $VO_n$ was highlighted with colored polyhedrons.

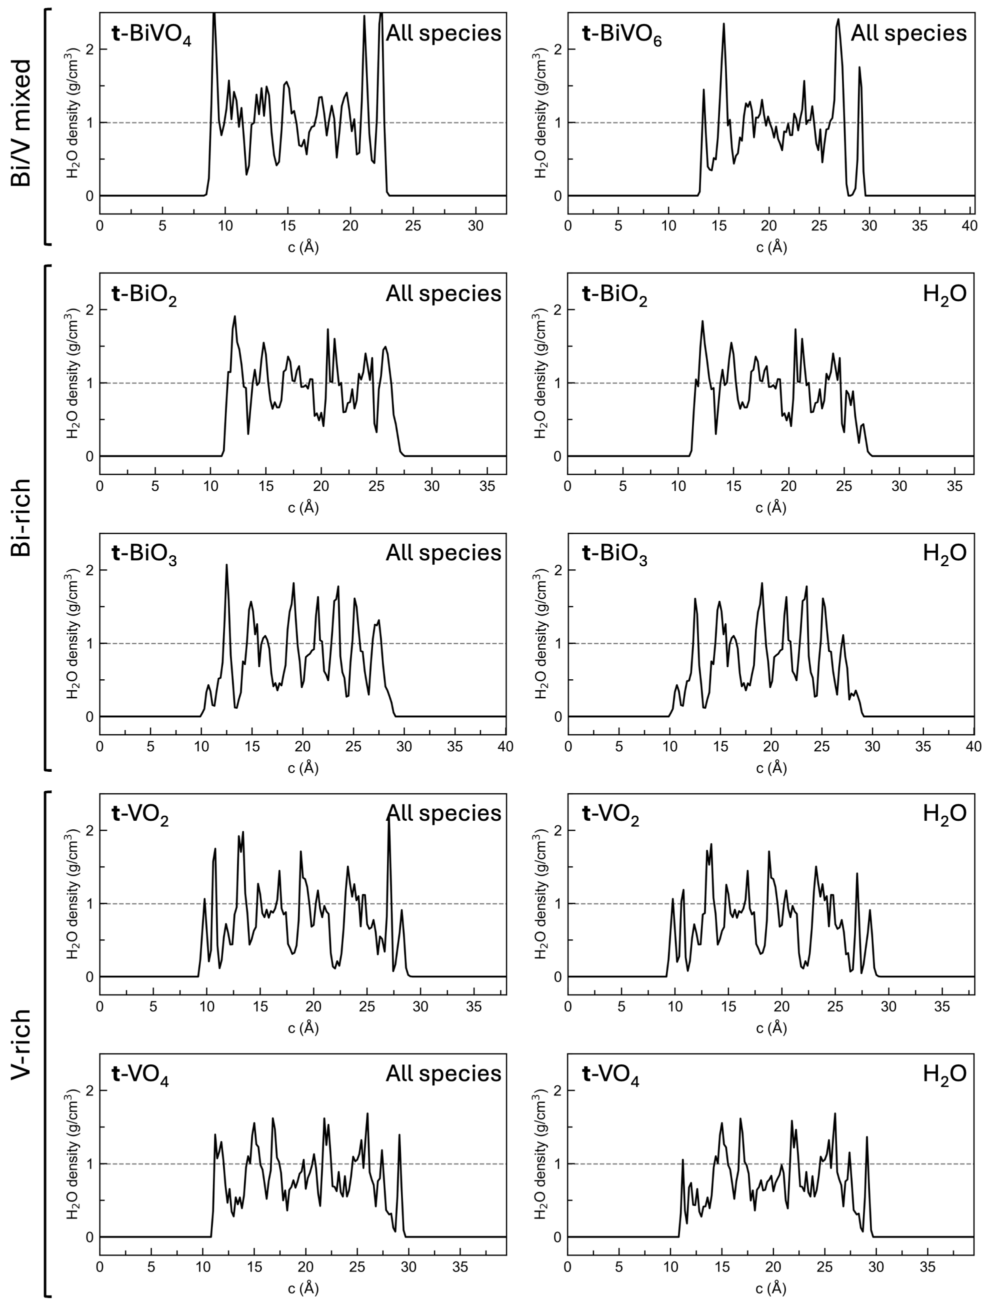


Figure S4: Water density plots from *ai*MD trajectories for Bi/V mixed, Bi-rich, and V-rich interfaces as a function of the c-axis perpendicular to the interface. "All species" includes all water-related species, i.e., $H_2O$, $^*OH$, $^*H$, and $H_3O^+$, while "$H_2O$" refers specifically to the density of $H_2O$ molecules in the trajectory.

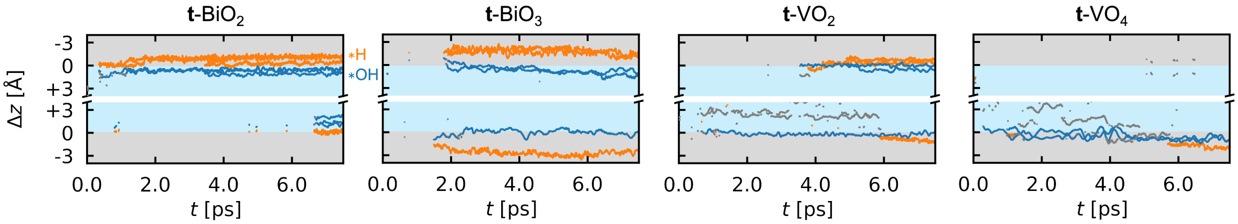


Figure S5: The time-dependent evolution of the relative z-coordinate position with respect to the $BiVO_4$/water interface is illustrated for $H^+$, $OH^-$, and other intermediate species using orange, blue, and dark gray markers, respectively. The surface and water regions are depicted in blue and light gray, respectively.

# References


(1) Bartók, A. P.; Payne, M. C.; Kondor, R.; Csányi, G. Gaussian Approximation Potentials: The Accuracy of Quantum Mechanics, without the Electrons. *Phys. Rev. Lett.* **2010**, *104*, 136403.

(2) Deringer, V. L.; Caro, M. A.; Csányi, G. Machine Learning Interatomic Potentials as Emerging Tools for Materials Science. *Adv. Mater.* **2019**, *31*, 1902765.

(3) Deringer, V. L.; Bartók, A. P.; Bernstein, N.; Wilkins, D. M.; Ceriotti, M.; Csányi, G. Gaussian Process Regression for Materials and Molecules. *Chem. Rev.* **2021**, *121*, 10073–10141.

(4) Timmermann, J.; Lee, Y.; Staacke, C. G.; Margraf, J. T.; Scheurer, C.; Reuter, K. Data-Efficient Iterative Training of Gaussian Approximation Potentials: Application to Surface Structure Determination of Rutile $IrO_2$ and $RuO_2$. *J. Chem. Phys.* **2021**, *155*, 244107.

(5) Bartók, A. P.; Kondor, R.; Csányi, G. On Representing Chemical Environments. *Phys. Rev. B* **2013**, *87*, 184115.

(6) Plimpton, S. Fast Parallel Algorithms for Short-Range Molecular Dynamics. *J. Comput. Phys.* **1995**, *117*, 1–19.

(7) Swope, W. C.; Andersen, H. C.; Berens, P. H.; Wilson, K. R. A Computer Simulation Method for the Calculation of Equilibrium Constants for the Formation of Physical Clusters of Molecules: Application to Small Water Clusters. *J. Chem. Phys.* **1982**, *76*, 637–649.

(8) Berendsen, H. J. C.; van Postma, J. P. M.; van Gunsteren, W. F.; DiNola, A.; Haak, J. R. Molecular Dynamics with Coupling to an External Bath. *J. Chem. Phys.* **1984**, *81*, 3684–3690.

(9) Hamann, D. R. Optimized Norm-Conserving Vanderbilt Pseudopotentials. *Phys. Rev. B* **2013**, *88*, 085117.

(10) Giannozzi, P. et al. Quantum ESPRESSO: A Modular and Open-Source Software Project for Quantum Simulations of Materials. *J. Phys. Condens. Matter* **2009**, *21*, 395502.

(11) Perdew, J. P.; Burke, K.; Ernzerhof, M. Generalized Gradient Approximation Made Simple. *Phys. Rev. Lett.* **1996**, *77*, 3865–3868.

(12) Dudarev, S. L.; Botton, G. A.; Savrasov, S. Y.; Humphreys, C. J.; Sutton, A. P. Electron-Energy-Loss Spectra and the Structural Stability of Nickel Oxide: An LSDA+$U$ Study. *Phys. Rev. B* **1998**, *57*, 1505.

(13) Seo, H.; Ping, Y.; Galli, G. Role of Point Defects in Enhancing the Conductivity of $BiVO_4$. *Chem. Mater.* **2018**, *30*, 7793–7802.

(14) Wang, W.; Strohbeen, P. J.; Lee, D.; Zhou, C.; Kawasaki, J. K.; Choi, K.-S.; Liu, M.; Galli, G. The Role of Surface Oxygen Vacancies in $BiVO_4$. *Chem. Mater.* **2020**, *32*, 2899–2909.

(15) Lee, D.; Wang, W.; Zhou, C.; Tong, X.; Liu, M.; Galli, G.; Choi, K.-S. The Impact of Surface Composition on the Interfacial Energetics and Photoelectrochemical Properties of $BiVO_4$. *Nat. Energy* **2021**, *6*, 287–294.

(16) Hilbrands, A. M.; Zhang, S.; Zhou, C.; Melani, G.; Wi, D. H.; Lee, D.; Xi, Z.; Head, A. R.; Liu, M.; Galli, G.; Choi, K.-S. Impact of Varying the Photoanode/Catalyst Interfacial Composition on Solar Water Oxidation: The Case of $BiVO_4(010)$/FeOOH Photoanodes. *J. Am. Chem. Soc.* **2023**, *145*, 23639–23650.

(17) Broyden, C. G. The Convergence of a Class of Double-Rank Minimization Algorithms: 2. The New Algorithm. *IMA J. Appl. Math.* **1970**, *6*, 222–231.

(18) Goldfarb, D. A Family of Variable-Metric Methods Derived by Variational Means. *Math. Comput.* **1970**, *24*, 23–26.

(19) Shanno, D. F. Conditioning of Quasi-Newton Methods for Function Minimization. *Math. Comput.* **1970**, *24*, 647–656.

(20) Kühne, T. D.; Iannuzzi, M.; Del Ben, M.; Rybkin, V. V.; Seewald, P.; Stein, F.; Laino, T.; Khaliullin, R. Z.; Schütt, O.; Schiffmann, F.; others CP2K: An Electronic Structure and Molecular Dynamics Software Package–Quickstep: Efficient and Accurate Electronic Structure Calculations. *J. Chem. Phys.* **2020**, *152*, 194103.

(21) Guidon, M.; Hutter, J.; VandeVondele, J. Robust Periodic Hartree-Fock Exchange for Large-Scale Simulations Using Gaussian Basis Sets. *J. Chem. Theory Comput.* **2009**, *5*, 3010–3021.

(22) Guidon, M.; Hutter, J.; VandeVondele, J. Auxiliary Density Matrix Methods for Hartree-Fock Exchange Calculations. *J. Chem. Theory Comput.* **2010**, *6*, 2348–2364.

(23) Wiktor, J.; Reshetnyak, I.; Ambrosio, F.; Pasquarello, A. Comprehensive Modeling of the Band Gap and Absorption Spectrum of $BiVO_4$. *Phys. Rev. Mater.* **2017**, *1*, 022401.

(24) Ambrosio, F.; Wiktor, J. Strong Hole Trapping due to Oxygen Dimers in $BiVO_4$: Effect on the Water Oxidation Reaction. *J. Phys. Chem. Lett.* **2019**, *10*, 7113–7118.

(25) Goedecker, S.; Teter, M.; Hutter, J. Separable Dual-Space Gaussian Pseudopotentials. *Phys. Rev. B* **1996**, *54*, 1703.

(26) VandeVondele, J.; Hutter, J. Gaussian Basis Sets for Accurate Calculations on Molecular Systems in Gas and Condensed Phases. *J. Chem. Phys.* **2007**, *127*, 114105.

(27) Wiktor, J.; Pasquarello, A. Electron and Hole Polarons at the $BiVO_4$–Water Interface. 2019; `https://doi.org/10.24435/materialscloud:2019.0035/v1`.

(28) Grimme, S.; Antony, J.; Ehrlich, S.; Krieg, H. A Consistent and Accurate Ab Initio Parametrization of Density Functional Dispersion Correction (DFT-D) for the 94 Elements H-Pu. *J. Chem. Phys.* **2010**, *132*.

(29) Larsen, A. H.; Mortensen, J. J.; Blomqvist, J.; Castelli, I. E.; Christensen, R.; Dułak, M.; Friis, J.; Groves, M. N.; Hammer, B.; Hargus, C.; others The Atomic Simulation Environment–A Python Library for Working with Atoms. *J. Phys.: Condens. Matter.* **2017**, *29*, 273002.

(30) Persson, K. A.; Waldwick, B.; Lazic, P.; Ceder, G. Prediction of Solid-aqueous Equilibria: Scheme to Combine First-principles Calculations of Solids with Experimental Aqueous States. *Phys. Rev. B* **2012**, *85*, 235438.

(31) Groß, A. Reversible vs Standard Hydrogen Electrode Scale in Interfacial Electrochemistry from a Theoretician's Atomistic Point of View. *J. Phys. Chem. C* **2022**, *126*, 11439–11446.

(32) Reuter, K. Ab Initio Thermodynamics and First-Principles Microkinetics for Surface Catalysis. *Catal. Lett.* **2016**, *146*, 541–563.

(33) Lee, T.; Soon, A. The Rise of Ab Initio Surface Thermodynamics. *Nat. Catal.* **2024**, *7*, 4–6.

(34) Reuter, K.; Scheffler, M. Composition, Structure, and Stability of $RuO_2(110)$ as a Function of Oxygen Pressure. *Phys. Rev. B* **2001**, *65*, 035406.

(35) Opalka, D.; Scheurer, C.; Reuter, K. Ab Initio Thermodynamics Insight into the Structural Evolution of Working $IrO_2$ Catalysts in Proton-Exchange Membrane Electrolyzers. *ACS Catal.* **2019**, *9*, 4944–4950.

(36) Irikura, K. K. Experimental Vibrational Zero-Point Energies: Diatomic Molecules. *J. Phys. Chem. Ref. Data* **2007**, *36*, 389–397.

(37) Benedict, W. S.; Gailar, N.; Plyler, E. K. Rotation-Vibration Spectra of Deuterated Water Vapor. *J. Chem. Phys.* **1956**, *24*, 1139–1165.

(38) Chase Jr., M.; NIST Standard Reference Data Program NIST-JANAF Thermochemical Tables. `https://doi.org/10.18434/T42S31`, 1998.

(39) Nørskov, J. K.; Rossmeisl, J.; Logadottir, A.; Lindqvist, L. R. K. J.; Kitchin, J. R.; Bligaard, T.; Jonsson, H. Origin of the Overpotential for Oxygen Reduction at a Fuel-Cell Cathode. *J. Phys. Chem. B* **2004**, *108*, 17886–17892.

(40) Milazzo, G.; Caroli, S.; Sharma, V. K. *Tables of Standard Electrode Potentials*; Wiley: Chichester, 1978.

(41) Bard, A. J.; Parsons, R.; Jordan, J. *Standard Potentials in Aqueous Solutions*; Marcel Dekker: New York, 1985.

(42) Bratsch, S. G. Standard Electrode Potentials and Temperature Coefficients in Water at 298.15 K. *J. Phys. Chem. Ref. Data* **1989**, *18*, 1–21.
